# Supplementary material for: Rethinking Distance Metrics for Counterfactual Explainability
Source: arXiv:2410.14522 source file (2024-10-18)
Supplement: Supplementary file 1 [file dataset_choice.tex]

\section{Dataset Details}
\label{app:datasets}

In this section, we provide both details on each of the datasets chosen for our MTurk survey, and additional information on what each dataset evaluates in terms of our results. Preprocessing information can be found in Appendix \ref{app:reproducibility}

\xhdr{Lucas \cite{guyon2008design}}
LUCAS is a synthetic dataset of $2000$ instances in which the binary outcome, whether or not an individual has lung cancer, is based on 11 other binary features: `Anxiety', `Peer Pressure', `Born on an Even Day', `Smoking', `Yellow Fingers', `Genetics', `Allergy', `Coughing', `Fatigue', `Attention Disorder', and `Car Accident'. The relationships and outcome are related through a provided causal graph with known conditional probabilities (see Appendix \ref{fig:lucas_causal_dag}). 

Due to the complete knowledge of the conditional probabilities and the small size of the feature set, we are able to convey the exact causal relationships to the survey participants, and verify whether their justifications for preferring one explanation over another accurately reflects these probabilities. For example, a participant may remark that `Smoking' is unlikely without `Anxiety' and `Peer Pressure'. This in turn allows us to examine how exact knowledge of a system correlates with an individual's preferences for certain types of explanations.

\xhdr{Adult \cite{Dua:2019}}

Adult is a well-known dataset from the UCI data repository which consists of $48842$ instances with 8 categorical features and 6 continuous for the purpose of predicting whether or not an individual made over \$50,000 in income as provided by the 1994 US Census. 

In order to introduce causal relationships in the Adult dataset, we use the graph from \citet{zhang2016causal} with an additional edge from `native-country' to `race' (We provide the considered DAG in Appendix \ref{fig:adult_causal_dag}). During preprocessing we discard: `fnlwgt', `education-num', `capital-gain', and `capital loss' due to their exclusion from the DAG provided by prior work. Additionally, we define `race', `sex',  and `native-country' as immutable features, and `relationship' as a mutable-nonactionable column due to its dependency on marital status and sex.

As this dataset is a mixture of continuous and categorical variables, we are able to investigate how the approach in Appendix \ref{app:complex} fits to data on very different scales. Moreover, unlike in the LUCAS case, we do not provide survey respondents with the causal relationships, and instead investigate the extent to which their personal beliefs on the way social systems function influence the explanations.

\xhdr{German Credit \cite{Dua:2019}} 
Similarly to the Adult dataset, German credit is another well-known dataset in the UCI repository with $1000$ instances and a combination of $20$ continuous and categorical features. However, unlike Adult and LUCAS, we do not have an underlying causal DAG for German Credit, so all variables are treated as independent. Additionally, we apply a log transform to `Credit amount', `Duration in months', and `Age in years', while also defining `Personal status and sex', `Purpose', and `Foreign worker' fields as immutable. Lastly, the `Property' field is discarded as the categories are not independent of one another.

German Credit provides an interesting setting in which we have a fairly small dataset with a great deal of complexity. Like in the adult dataset, this allows us to investigate cases in which participants have pre-existing understanding of how lending systems work. Yet, as we do not have information on the causal relationships, we are able to see how each approach handles uncertainty and we can determine whether this effect is noticeable to participants.
