# Supplementary material for: Rethinking Distance Metrics for Counterfactual Explainability
Source: arXiv:2410.14522 source file (2024-10-18)
Supplement: Supplementary file 2 [file figures.tex]

\section{Causal Map of the UCI Adult Dataset}
\label{fig:adult_causal_dag}

\begin{figure}
    \centering
    \includegraphics[scale=0.45]{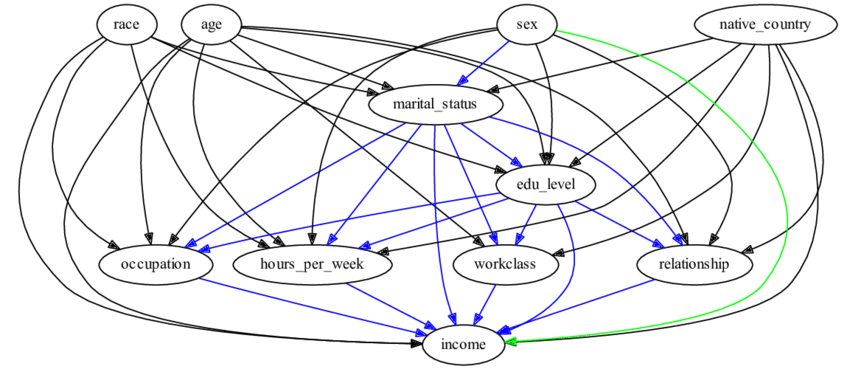}
    \caption{Casual graph for the UCI Adult Dataset. Not included here is the added edge going from native-country to race. Reprinted from: Zhang, L., Wu, Y., \& Wu, X. (2017). A Causal Framework for Discovering and Removing Direct and Indirect Discrimination. 10.24963/ijcai.2017/549. }
\end{figure}

\newpage
\section{Causal Map of the LUCAS Dataset}
\label{fig:lucas_causal_dag}

\begin{figure}
    \centering
    \includegraphics[scale=0.2]{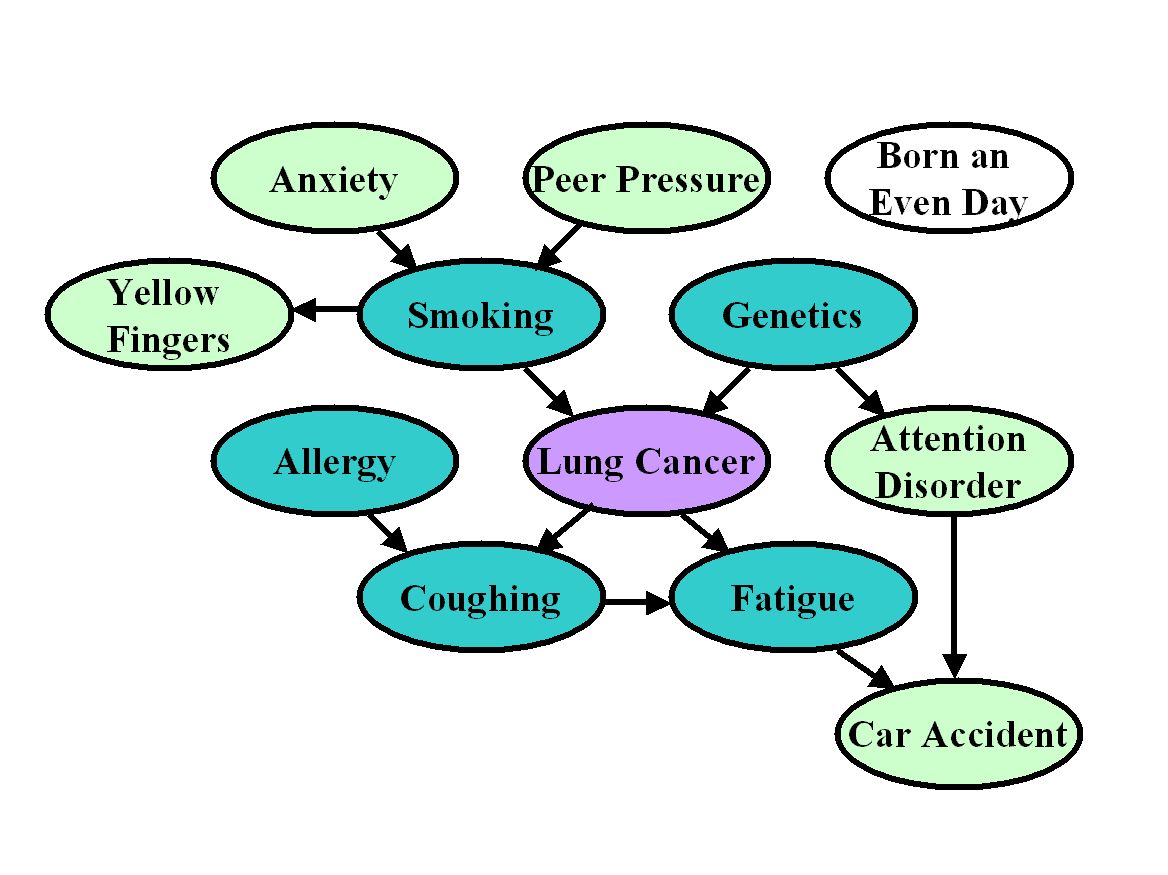}
    \caption{Casual graph for the LUCAS Dataset. Reprinted from: Guyon, I., Aliferis, C., Cooper, G., Elisseeff, A., Pellet, J. P., Spirtes, P., \& Statnikov, A. (2008, December). Design and analysis of the causation and prediction challenge. In Causation and Prediction Challenge (pp. 1-33). PMLR. }
\end{figure}

\newpage
\section{Survey Instructions}
\label{app:survey_instructions}

\subsection{\centering Participant Information for LUCAS Dataset \cite{guyon2008design}}
\label{app:lucas_survey_screen}
\begin{figure}[h!]
    \centering
    \includegraphics[scale=0.8]{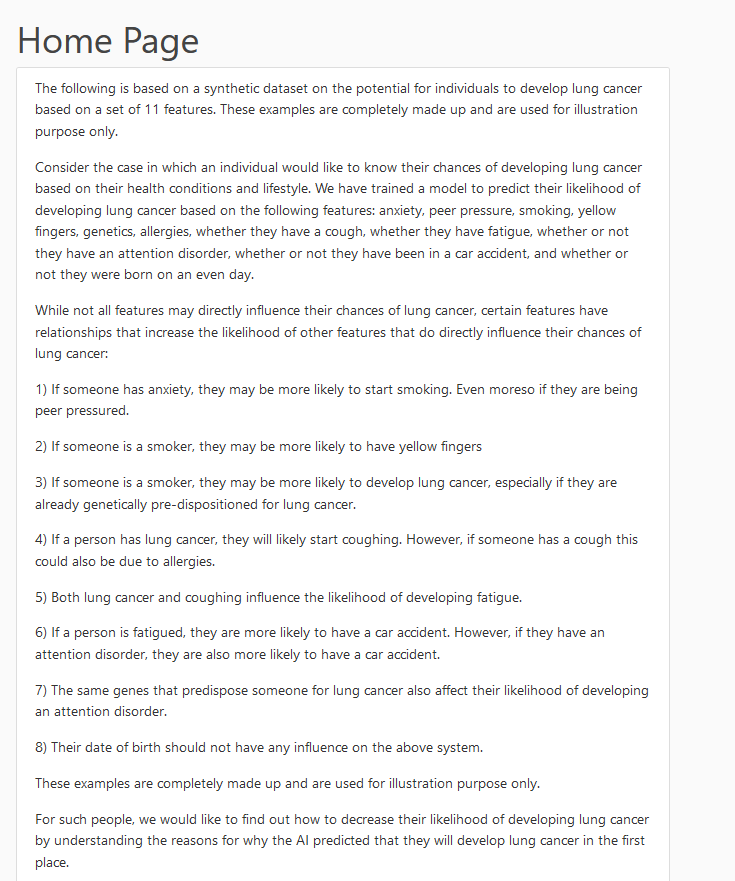}
    \caption{Information shown to participants who provide preferences on the LUCAS dataset}
\end{figure}

\newpage
\subsection{\centering Participant Information for German Credit Dataset \cite{Dua:2019}}
\label{app:german_survey_screen}
\begin{figure}[h!]
    \centering
    \includegraphics[scale=0.8]{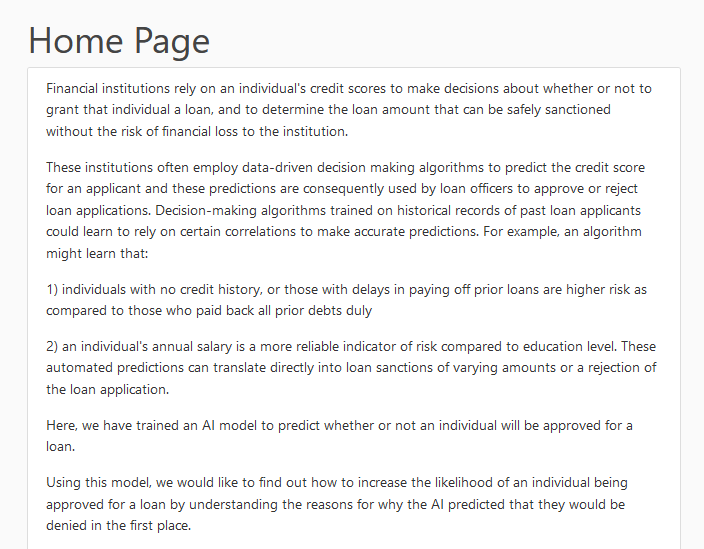}
    \caption{Information shown to participants who provide preferences on the German Credit dataset}
\end{figure}

\newpage
\subsection{\centering Participant Information for Adult Income Dataset \cite{Dua:2019}}
\label{app:adult_survey_screen}
\begin{figure}[h!]
    \centering
    \includegraphics[scale=0.6]{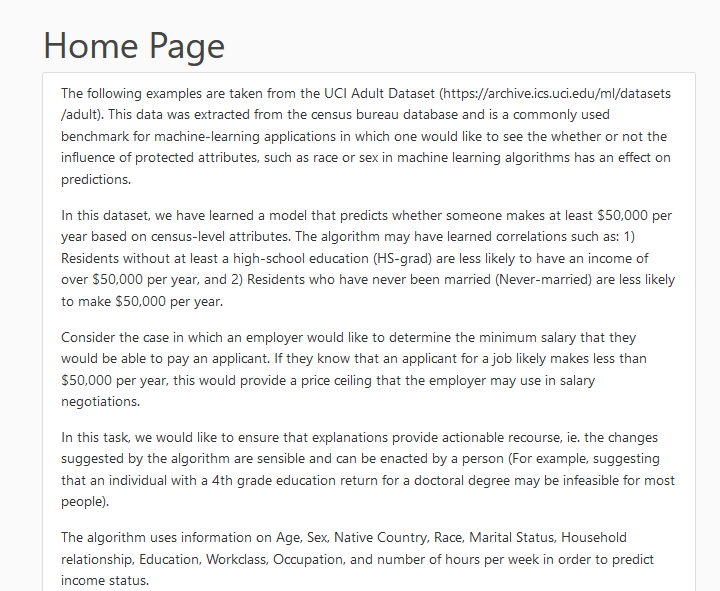}
    \caption{Information shown to participants who provide preferences on the Adult Income dataset}
\end{figure}

\newpage
\subsection{\centering Example Survey Screen}
\label{app:survey_screen}
\begin{figure}[h!]
    \centering
    \includegraphics[scale=0.6]{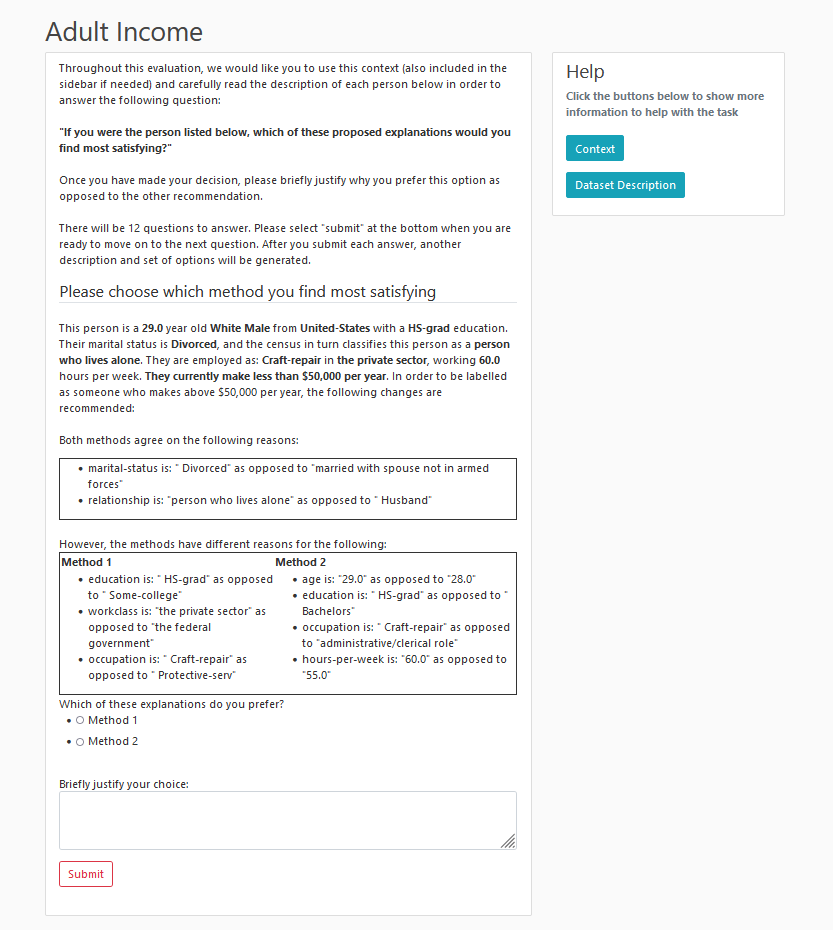}
    \caption{Example of a screen from the survey}
\end{figure}

\newpage
\section{IRB Approval}
\label{app:irb}

Due to double-blind review process, we excluded the IRB approval form in the initial submission. If accepted, we will include the IRB Approval form here.
