# Supplementary material for: Rethinking Distance Metrics for Counterfactual Explainability
Source: arXiv:2410.14522 source file (2024-10-18)
Supplement: Supplementary file 3 [file laplace_derivation.tex]

\section{Derivation of Counterfactual Posterior wrt Laplace Approximation}
\label{app:derivation_laplace}

In \ref{sec_complex}, \ref{sec_cf_decode}, we showed that we can use a Laplace Approximation in order to learn a new prior, $g( x' )$, for the counterfactual points, $x'$, in which for $x' \sim g$ implies $f( x' ) = y'$, where $y'$ is the desired predicted output. In this section, we derive the form of the counterfactual distribution, $p( x' | x ) \propto p( x | x' ) g( x' )$.

Reiterating from Appendix \ref{app:derivation_pgm2}, the conditional distribution, $p( \vx | \vx' )$ is,
\begin{equation*}
    \mathcal{N}( \mu + W \Lambda ( \vx' - \mu ), \Lambda^{-1} - W \Lambda W^{T} )
\end{equation*}
where the joint distribution, $p( x', x ) = \mathcal{N}\big( \begin{bmatrix} \mu \\ \mu \end{bmatrix}, \begin{bmatrix} \Lambda^{-1} & W \\ W^{T} & \Lambda^{-1} \end{bmatrix} \big)$. In addition, let $g( x' ) = \mathcal{N}( \mu_{x'}, \Lambda_{x'}^{-1} )$. Then, the negative log probability of their joint distribution distribution, $g( x', x )$ is,

\begin{align*}
    - \log g( x', x ) &= - \log p( x | x' ) - \log g( x' ) \\
    &= ( x - \mu_{x|x'} )^{T} \Lambda_{x|x'} ( x - \mu_{x|x'} ) + ( x' - \mu_{x'} )^{T} \Lambda_{x'} ( x' - \mu_{x'} ) \\
    &= x^{T} \Lambda_{x|x'} x - 2 x^{T} \Lambda_{x|x'} \mu_{x|x'} + \mu_{x|x'}^{T} \Lambda_{x|x'} \mu_{x|x'} + x'^{T} \Lambda_{x'} x' - 2 x'^{T} \Lambda_{x'} \mu_{x'} + \mu_{x'}^{T} \Lambda_{x'} \mu_{x'} \\
    &= x^{T} \Lambda_{x|x'} x - 2 x^{T} \Lambda_{x|x'} \mu_{x|x'} + \mu_{x|x'}^{T} \Lambda_{x|x'} \mu_{x|x'} + x'^{T} \Lambda_{x'} x' - 2 x'^{T} \Lambda_{x'} \mu_{x'} + c \\
\end{align*}

We first focus on the quadratic terms. Note that $\mu_{x|x'}$ is a function of $x'$, so $ x^{T} \Lambda_{x|x'} \mu_{x|x'}$ and $\mu_{x|x'}^{T} \Lambda_{x|x'} \mu_{x|x'} $ are not immediately linear/constant respectively.

\begin{align*}
    &- \log g( x' , x ) \propto - \log p( x | x' ) - \log g( x' ) \\
    &= x^{T} \Lambda_{x|x'} x - 2 x^{T} \Lambda_{x|x'} \mu_{x|x'} + \mu_{x|x'}^{T} \Lambda_{x|x'} \mu_{x|x'} + x'^{T} \Lambda_{x'} x' + ... \\
    &= x^{T} \Lambda_{x|x'} x - 2 x^{T} \Lambda_{x|x'} ( \mu + W \Lambda ( x' - \mu ) ) + ( \mu + W \Lambda ( x' - \mu ) )^{T} \Lambda_{x|x'} ( \mu + W \Lambda ( x' - \mu ) ) + x'^{T} \Lambda_{x'} x' + ... \\
    &= x^{T} \Lambda_{x|x'} x - 2 x^{T} \Lambda_{x|x'} \mu - 2  x^{T} \Lambda_{x|x'} W \Lambda ( x' - \mu ) + \mu^{T} \Lambda_{x|x'} \mu + 2 ( W \Lambda ( x' - \mu ) )^{T} \Lambda_{x|x'} \mu \\
    &\hspace{2cm} + ( W \Lambda ( x' - \mu ) )^{T} \Lambda_{x|x'} ( W \Lambda ( x' - \mu ) ) + x'^{T} \Lambda_{x'} x' + ... \\
\end{align*}
Since we're only focused on the quadratic case for now, we drop $\mu^{T} \Lambda_{x|x'} \mu $, $2 x^{T} \Lambda_{x|x'} \mu$, and $2 ( W \Lambda ( x' - \mu ) )^{T} \Lambda_{x|x'} \mu $ as they are constant/linear.

\begin{align*}
    &= x^{T} \Lambda_{x|x'} x - 2  x^{T} \Lambda_{x|x'} W \Lambda ( x' - \mu ) + ( W \Lambda ( x' - \mu ) )^{T} \Lambda_{x|x'} ( W \Lambda ( x' - \mu ) ) + x'^{T} \Lambda_{x'} x' + ... \\
    &= x^{T} \Lambda_{x|x'} x  - 2 x^{T} \Lambda_{x|x'} W \Lambda x' + 2  x^{T} \Lambda_{x|x'} W \Lambda \mu + x' \Lambda W \Lambda_{x|x'} W \Lambda x' \\
    &\hspace{2cm} - 2 x' \Lambda W \Lambda_{x|x'} W \Lambda \mu + \mu^{T} \Lambda W \Lambda_{x|x'} W \Lambda \mu + x'^{T} \Lambda_{x'} x'
\end{align*}

Again, disregarding the non-quadratic terms, $2  x^{T} \Lambda_{x|x'} W \Lambda \mu$, $2 x' \Lambda W \Lambda_{x|x'} W \Lambda \mu$, and $\mu^{T} \Lambda W \Lambda_{x|x'} W \Lambda \mu$,

\begin{align*}
     &= x^{T} \Lambda_{x|x'} x  - 2 x^{T} \Lambda_{x|x'} W \Lambda x' + x'^{T} \Lambda W \Lambda_{x|x'} W \Lambda x' + x'^{T} \Lambda_{x'} x' \\
     &= x^{T} \Lambda_{x|x'} x  - 2 x^{T} \Lambda_{x|x'} W \Lambda x' + x'^{T} ( \Lambda_{x'} + \Lambda W \Lambda_{x|x'} W \Lambda ) x' \\
\end{align*}

Thus the inverse covariance of $g( x', x ) $, is: $\Lambda_{x,x'} = \begin{bmatrix} \Lambda_{x|x'} & - \Lambda_{x|x'} W \Lambda \\ ( - \Lambda_{x|x'} W \Lambda )^{T} & \Lambda_{x'} + \Lambda W \Lambda_{x|x'} W \Lambda \end{bmatrix}$, where $\Lambda_{x|x'} = ( \Lambda^{-1} - W \Lambda W^{T} )^{-1}$.

\jwcomment{Go back through and add in $\frac{1}{2} \times$ stuff}

We now focus on the linear terms as, $x \Sigma^{-1} \mu \implies \mu = \Sigma \Sigma^{-1} \mu$.

\begin{align*}
    g( x, x' ) &= ... - 2 x^{T} \Lambda_{x|x'} \mu + 2 x^{T} \Lambda_{x|x'} W \Lambda \mu + 2 \mu^{T} \Lambda_{x|x'} W \Lambda x' ) \\
    &\hspace{2cm} - 2 x' \Lambda W \Lambda_{x|x'} W \Lambda \mu - 2 x'^{T} \Lambda_{x'} \mu_{x'} \\
    &= - 2 x^{T} ( \Lambda_{x|x'} \mu - \Lambda_{x|x'} W \Lambda \mu ) \\
    &\hspace{2cm} + 2 x'^{T} ( \Lambda W \Lambda_{x|x'} \mu - \Lambda W \Lambda_{x|x'} W \Lambda \mu - \Lambda_{x'} \mu_{x'} ) \\
\end{align*}

Thus, the mean of $g( x, x' )$ is, $\mu_{x,x'} = \Lambda_{x,x'}^{-1} \begin{bmatrix} ( - \Lambda_{x|x'} \mu + \Lambda_{x|x'} W \Lambda \mu ) \\ \Lambda W \Lambda_{x|x'} \mu - \Lambda W \Lambda_{x|x'} W \Lambda \mu - \Lambda_{x'} \mu_{x'} \end{bmatrix}$

From here, we can find the counterfactual distribution using Eq.~\eqref{cond_mu} and Eq.~\eqref{cond_cov} for the new $\mu_{x,x'}$ and $\Lambda_{x,x'}$.
