# Supplementary material for: Rethinking Distance Metrics for Counterfactual Explainability
Source: arXiv:2410.14522 source file (2024-10-18)
Supplement: Supplementary file 4 [file limitations.tex]

\section{Human-Subjects Study Limitations}
\label{app:limitations}

Regarding the AMT surveys, due to the associated costs of incentivizing attentive participation, we were unable to increase the sample size to levels that would more clearly show statistically significant preferences. Moreover, during pilot testing, we found that the quality of participant responses decreased significantly after approximately 14 questions. In order to ensure that we received high quality results, we limited the survey to only 12 questions. As such, we limited the number of baseline evaluation methods to three. Through simulation, we found that three comparison methods was the maximum number of methods that ensures that we can differentiate between participants responding randomly in bad faith, and participants with genuine preferences in methodology. Still, due to the number of respondents who did not complete the survey in good faith, we had to discard approximately $25\%$ of responses ($~500$ comparisons) which further limits the clarity of general statements about the methodologies. 

Of the participants that were included in the study, we had a high representation of people who identified as men ($70\%$), those who self identify as White ($78\%$), those with graduate degrees ($48\%$), and those with ages between $26$ and $40$ ($60\%$). Thus, the generalizations that are based around the understanding and preferences of these groups.
